# Supplementary material for: The Foes of Neural Network's Data Efficiency Among Unnecessary Input Dimensions
Source: arXiv:2107.06409 source file (2021-07-13)
Supplement: Supplementary file 1 [file supplementary_dcnn.tex]

\input{app_deep_cnn}
